# Supplementary material for: Robust resonant anomaly detection with NPLM
Source: arXiv:2501.01778 source file (2025-01-03)
Supplement: Supplementary file 1 [file appendix.tex]

\subsection{BDT sensitivity to hyperparameters selection}\label{app:bdt}
We present the results of our experiments with various hyperparameters choice in Figure~\ref{fig:BDT-variance-res}. Each row in the figure is produced using a different set of hyperparameters, while each column corresponds to a different amount of resonant signal injection.
The power curves in the figure highlight the variance of the detection power due to the hyperparameter choice. In particular, hyperparameters that are optimal for large signal injection become blind to low signal injection. The anomaly selection threshold $\rm thr$ seems to play a critical role.

Moreover, we run the BDT classifiers over the non-resonant signal benchmark and report similar results in Figure~\ref{fig:BDT-variance-non-res}. By comparing each row of the two figures, we notice that the best model for a non-resonant signal performs poorly on a resonant signal, in particular at low signal injections.

These results highlight the criticality of the model selection step in the anomaly detection strategy and the need for a systematic approach that is robust to variations of signal strength and shape. 
\begin{comment}
\begin{figure}[h]
    \centering
    %\includegraphics[width=\linewidth]{figures/BDTsqrt_powers_resample.pdf}\\
    \includegraphics[width=\linewidth]{figures/data_BDTsqrt_leaf100_lambda1e-1_thrs_powers_resample.pdf}\\
    \includegraphics[width=\linewidth]{figures/data_BDTsqrt_leaf100_lambda1e-2_thrs_powers_resample.pdf}\\
    \includegraphics[width=\linewidth]{figures/data_BDTsqrt_leaf31_lambda1e-1_thrs_powers_resample.pdf}\\
    \includegraphics[width=\linewidth]{figures/data_BDTsqrt_leaf31_lambda1e-2_thrs_powers_resample.pdf}
    \caption{\textbf{BDT-classifier. Resonant signal} Discovery power of a cut-and-count signal-agnostic test on the classifier score based on BDT ....}
    \label{fig:BDT-variance-res}
\end{figure}
\end{comment}
\begin{figure}[h]
    \centering
    \includegraphics[width=\linewidth]{figures/extra-data_BDTsqrt_leaf100_lambda1e-1_thrs_powers_resample.pdf}\\
    \includegraphics[width=\linewidth]{figures/extra-data_BDTsqrt_leaf100_lambda1e-2_thrs_powers_resample.pdf}\\
    \includegraphics[width=\linewidth]{figures/extra-data_BDTsqrt_leaf31_lambda1e-1_thrs_powers_resample.pdf}\\
    \includegraphics[width=\linewidth]{figures/extra-data_BDTsqrt_leaf31_lambda1e-2_thrs_powers_resample.pdf}
    \caption{\textbf{BDT-classifier. Non-resonant signal} Discovery power of a cut-and-count signal-agnostic test on the classifier score based on BDT.}
    \label{fig:BDT-variance-non-res}
\end{figure}
\subsection{NPLM sensitivity to hyperparameters selection}\label{app:nplm}
The NPLM strategy provides an alternative approach to test for anomalies that is less sensitive to hyperparameters choice. Being an end-to-end approach from the data to the statistical test, it does not require an anomaly selection stage, eliminating the variance introduced in CwoLa-like methods by the selection threshold $\rm thr$. Moreover, a multiple test strategy has been recently introduced to mitigate the impact of hyperparameters~\cite{Grosso:2024wj}.
We run NPLM on the same signal benchmarks considered for the BDT, using as input variables the five features given to the BDT plus the resonant variable\footnote{The resonant variable is given as an additional input because the NPLM method computes the test final test in a single step.}. Also in this case, we run different model configurations, varying the two main hyperparameters of the strategy, namely the number of kernels $M$ and the L2 regularization magnitude $\lambda$.
Figure~\ref{fig:NPLM-variance} presents the power curves for the NPLM test for both the resonant (top row) and the non-resonant (bottom row) signals. The spread of power curves is significantly reduced and the performances among different signal scenarios and amount of injection is stable.
\begin{figure}[t]
    \centering
    \includegraphics[width=\linewidth]{figures/NPLM6Dt_powers_new.pdf}
    \includegraphics[width=\linewidth]{figures/extra-data_NPLM6Dt_powers_new.pdf}
    \caption{\textbf{KM-NPLM} Discovery power of kernel methods based NPLM classifiers computing the maximum-likelihood-ratio test. top: resonant; bottom: non-resonant signal}
    \label{fig:NPLM-variance}
\end{figure}

To better compare the spread of performance of the NPLM approach and the cut-and-count approach based on a BDT classifier, we report a summary of power curves for the resonant signal in Figure~\ref{fig:NPLM-BDT-variance}. 

%\begin{figure}
%    \centering
%    \includegraphics[width=1\linewidth]{figures/NPLM5Dt-BDT5Dssqrtb_thr0.99_powers_resample.pdf}
%    \caption{\textbf{BDT-classifier vs. NPLM-Neyman-Person test.}}
%    \label{fig:ssqrt}
%\end{figure}

\begin{comment}
\begin{figure}
    \centering
    \includegraphics[width=\linewidth]{figures/NPLM6D-BDTleaf31_l20_lr0.01_powers_resample.pdf}\\
    \includegraphics[width=\linewidth]{figures/NPLM6D-BDTleaf31_l20_lr0.1_powers_resample.pdf}\\
    \includegraphics[width=\linewidth]{figures/NPLM6D-BDTleaf100_l20_lr0.01_powers_resample.pdf}\\
    \includegraphics[width=\linewidth]{figures/NPLM6D-BDTleaf100_l20_lr0.1_powers_resample.pdf}\\
    \caption{\textbf{BDT-classifiers vs. KM-NPLM.} Discovery power of a cut-and-count signal-agnostic test on the classifier score based on BDT ... and kernel methods based NPLM classifiers}
    \label{fig:enter-label}
\end{figure}
\end{comment}

% \begin{itemize}
%     \item BDT as a function of hyperparameters
%     \item Do BDTs vary a lot? Probably
%     \item NPLM with kernel method with also hyperparameters.
%     \item choice of rejection threshold is itself a hyperparameter $\rightarrow$ How does this affect results?
%     \item NPLM can actually characterise the shape of the bump $\rightarrow$ demonstrate this.
\end{itemize}
